# Supplementary material for: Temporally-Aware Feature Pooling for Action Spotting in Soccer Broadcasts
Source: arXiv:2104.06779 source file (2021-04-14)
Supplement: Supplementary file 1 [file spotting-supplementary.tex]

\begin{table*}[ht]
\scriptsize
    \caption{\textbf{Leaderboard for action spotting} (Average-mAP \%). $^*$results obtained with our re-implementation and optimized training. In bold, the best performances per column, irrespective of the shown or unshown nature of the actions, for consistency with the table provided in the main paper.} 
    \centering
    \setlength{\tabcolsep}{2pt}
    % \tabcolsep{6pt}
    \resizebox{\linewidth}{!}{
    \begin{tabular}{l||c|c||c|c||c|c|c|c|c|c|c|c|c|c|c|c|c|c|c|c|c}
     &  \begin{turn}{90}SoccerNet-v1\end{turn}  &  \begin{turn}{90}SoccerNet-v2\end{turn} &  \begin{turn}{90}shown\end{turn}   &  \begin{turn}{90}unshown\end{turn}  & \begin{turn}{90} Ball out \end{turn} & \begin{turn}{90}Throw-in\end{turn} & \begin{turn}{90}Foul \end{turn} & \begin{turn}{90}Ind. free-kick \end{turn} & \begin{turn}{90}Clearance \end{turn} & \begin{turn}{90}Shots on tar. \end{turn} & \begin{turn}{90}Shots off tar. \end{turn} & \begin{turn}{90}Corner \end{turn} & \begin{turn}{90}Substitution \end{turn} & \begin{turn}{90}Kick-off \end{turn} & \begin{turn}{90}Yellow card \end{turn} & \begin{turn}{90}Offside \end{turn} & \begin{turn}{90}Dir. free-kick \end{turn} & \begin{turn}{90}Goal \end{turn} & \begin{turn}{90}Penalty \end{turn} & \begin{turn}{90}Yel.$\to$Red \end{turn} & \begin{turn}{90}Red card\end{turn} \\ 

       \midrule \midrule
Counts (test set)                   &   1369   & 22551 & 18641 & 3910 & 6460&	3809&	2414&	2283&	1631&	1175&	1058&	999&	579&	514&	431&	416&	382&	337&	41&	14&	8 \\ 

Counts shown & & & 18641 & & 6177&	2740&	2373&	1266&	777&	1170&	1055&	881&	472&	156&	365&	395&	395	&326&	41&	8&	14 \\

Counts unshown & & & & 3910 & 282&	1068&	40&	1017&	853&	1&	2&	118&	92	&357&	17	&21	&31	&0&	0&	0&	0 \\

\midrule \midrule

Rongved~\etal~\cite{rongved-ism2020}               & 32.0 & -    & -    & -    & -    & -    & -    & -    & -    & -    & -    & -    & -    & -    & -    & -    & -    & -    & -    & - & -   \\  \midrule
Vats~\etal~\cite{vats2020event}                   & 60.1 & -    & -    & -    & -    & -    & -    & -    & -    & -    & -    & -    & -    & -    & -    & -    & -    & -    & -    & -& -\\  \midrule \midrule

MaxPool~\cite{Giancola_2018_CVPR_Workshops}   & 31.1$^*$ & 17.5 & 18.6 & 15.2 & 45.4	&34.2&	33.9&	15.5&	14.0&	12.6&	14.1&	22.5&	30.3&	23.9&	13.3&	2.9&	6.0&	27.8&	0.7&	0.1&	0.1\\ 

MaxPool shown & & & 18.6 & &45.5&	35.3&	33.9&	14.2&	14.0&	12.6&	14.3&	22.6&	36.7&	31.5&	7.6&	3.6	&15.2&	27.8&	0.7&	0.1	&0.1 \\

MaxPool unshown & & & & 15.2 & 44.8&	28.3&	31.8&	18.5&	14.5&	1.6&	2.1&	24.2&	6.2&	20.7&	0.5&	0.5	&3.8&	-&	-&	-&	- \\

\midrule

NetVLAD~\cite{Giancola_2018_CVPR_Workshops}   & (49.7)/57.0$^*$ & 39.7 & 41.6 &\B30.1 & 56.5	&47.7&	51.4&	29.4&	40.3&	\B33.7&	\B35.7&	53.8&	\B54.6&	47.0&	\B45.0&	\B32.1&	34.4&	70.3&	37.9&	\B2.6&	\B3.2 \\

NetVLAD shown & & & 41.6 & & 56.7&	49.6&	51.7&	26.9&	48.7&	33.8&	35.8&	54.7&	60.3	&51.8	&39.5&	34.4&	48.6&	70.3&	37.9&	3.2&	2.6 \\

NetVLAD unshown & & & & 30.1 & 51.4	&44.0&	36.9&	34.3&	32.1&	2.7&	45.0&	48.4&	24.9&	45.5&	2.0&	19.0&	4.8&	-&	-&	-&	- \\ 

\midrule

AudioVid~\cite{Vanderplaetse2020Improved}   & 56.0 & 39.9    & \B43.0 & 23.3 & 54.3&	50.0&	\B55.5&	22.7&	46.7&	26.5&	21.4&	66.0&	54.0&	\B52.9&	35.2&	24.3&	\B46.7&	69.7&	\B52.1&	0.0&	0.0 \\ 

AudioVid shown & & & 43.0 & & 54.4&	55.5&	55.8&	21.2&	64.4&	26.5&	21.5&	70.5&	56.9&	67.9&	51.8&	25.1&	36.8&	69.7&	52.1&	0.0&	0.0 \\

AudioVid unshown & & & & 23.3& 48.6&	36.6&	23.9&	26.7&	29.1&	0.0&	0.0&	45.3&	23.1&	46.7&	1.1&	14.5&	6.4&	-&	-&	-&	- \\

\midrule

CALF~\cite{cioppa2020context}             &(\B62.5)/63.8$^*$ &\B40.7 &42.1 & 29.0 & \B63.9&	\B56.4&	53.0&	\B41.5&	\B51.6&	26.6&	27.3&	\B71.8&	47.3&	37.2&	41.7&	25.7&	43.5&	\B72.2&	30.6&	0.7&	0.7 \\ 

CALF shown	& & &42.1 & &64.1	&59.2	&53.5	&39.4	&59.4	&26.6	&27.4	&72.8	&57.2	&29.1	&49.3	&28.0	&45.5	&72.2	&30.6	&0.7	&0.7 \\

CALF unshown	& & & &29.0 	&58.9&	49.4&	28.3&	44.5&	46.2&	2.4	&10.0&	59.6&	16.0&	40.0&	3.8&	10.3&	7.1&	-&	-&	-&	- \\

\bottomrule 
% Avg. human                                  & -    & 80.5 & -    & -    & -    & -    & -    & -    & -    & -    & -    & -    & -    & -    & -    & -    & -    & -    & -    & -\\ 

    \end{tabular}}
    \label{tab:more-action-spotting}
\end{table*}
