# Supplementary material for: Temporally-Aware Feature Pooling for Action Spotting in Soccer Broadcasts
Source: arXiv:2104.06779 source file (2021-04-14)
Supplement: Supplementary file 2 [file 7_supplementary.tex]

% \section{Supplementary Material}

% \section{Supplementary: Results on \SN1.}

% We trained our NetVLAD++ module on the $3$ classes of \SN1 (\textit{goals}, \textit{subs} and \textit{cards}) yielding $62.7 \pm 0.4$ Average-mAP, yet falling $1.1\%$ short of CALF ($63.8\%$). Moreover, we compare our results with the NetVLAD optimized for the NMS and sliding window $T$, that yields $63.1\pm0.4$, $0.4\%$ better than NetVLAD, although within noise range. 

% First, it is worth noting that an optimized NetVLAD pooling module can reach similar performances than \CALF. 

% Second, NetVLAD++ does not further improve NetVLAD on \SN1, most probably due to the sparsity and scarcity of the supervisory action spots signals, with $\sim20\times$ less annotations in \SN1 w.r.t \SN2. 

% Finally, the learnable linear layer for feature projection also falls short w.r.t PCA on \SN1, with NetVLAD (+lin.layer) depicting a drop of $6.5\%$ ($55.7\pm0.5$) w.r.t its PCA counterpart. Again we argue the amount of supervision to be the cause of such drop in performances.

\section{Qualitative results}

\section{Code release}
